# Supplementary material for: Feasibility-Guided Safety-Aware Model Predictive Control for Jump Markov Linear Systems
Source: arXiv:2310.14116 source file (2024-09-15)
Supplement: Supplementary file 1 [file 7_Appendix.tex]

\section*{APPENDIX}

\subsection{Convexity of Safety-aware Trajectory Planning}

\begin{theorem}[Convex Safety-aware Trajectory Planning]
\label{theorem:qp}
Take a quadratic objective that includes a reference guidance cost term $\|(\pX_{k}^i-\pX_{r})\|^2_Q$ and a penalty on the control effort  $\|{\pU_k}\|^2_R$, where $Q, R \succ 0$. Further, represent the closed-loop dynamics as a JMLS, and the control barrier constraints as halfspaces.
Then, Problem \ref{prob:safetrajectoryplanning} is convex.    
\end{theorem}
\begin{proof}
Given weighting matrices $Q, R \succ 0$, $\mu_0(\cdot) \in [0,1]$, and $\sum_{i \in \mu_0} \mu_0(i) = 1$, the Hessian $\mathbf{H}$ of the objective function with respect to both $x$ and $u$ is positive definite. Thus, $ \mathbf{H} \phantom{.} J(x, u) = 
\nabla^{2} J(x, u) \succ 0$, and
therefore, the objective function is convex. Given the constraints are all linear, the feasible set is likewise convex. Thus, the above problem formulation is convex. 
\end{proof}

\begin{remark}
    The convexity of Problem \ref{prob:safetrajectoryplanning} is desirable for two reasons. First, since the solution to a convex OCP is a global minimum, we can guarantee solution optimality. Additionally, determining solution feasibility is only guaranteed in finite time for convex problems. Second, convex OCPs are more amenable to real-time execution. However, we note that our approach will still work for non-convex problems, only at the cost of global optimality and guaranteed computation time.
\end{remark}

\subsection{Feasbile Set Analysis}
% \qh{We need to define what $F_{k,consensus}$ and $F_{k,separate}$ are first if the Lemma is going to be worded like this.}
\begin{lemma}
Let the feasible control set under consensus be $\mathcal{F}_{k,\text{con}}$, and the set for independent control be $\mathcal{F}_{k,\text{ind}}$. Then the feasible set for Problem \ref{prob:safetrajectoryplanning} at horizon timestep $k$ under control consensus $\mathcal{F}_{k,\text{con}} \subseteq \mathcal{F}_{k,\text{ind}}$.
\label{lemma1}
\end{lemma}
\begin{proof}
From \eqref{eq:modesafeset}, we can reconstruct the set of control inputs that generated the mode-dependent safe set $\mathcal{S}_k^i$:
\begin{equation}
    {\mathcal{U}^i_{\mathcal{S}}}_k = \{\pU_{t+k}^i \in \mathbb{R}^{m}: \Delta{\beta}(\pX_k,\pU_k)\geq-\gamma\beta(\pX_k)\}
\end{equation}

The feasible set for a mode $i$ at horizon timestep $k$ is then the intersection of the safe control set ${\mathcal{U}^i_{\mathcal{S}}}_k$ and the allowable control set $\mathcal{U}$ defined in System \eqref{sys:linear}:
\begin{equation}
    \mathcal{F}_k^i = {\mathcal{U}^i_{\mathcal{S}}}_k \cap \phantom{.}\mathcal{U}
\end{equation}

In order to determine the mode-independent feasible set $\mathcal{F}_k$, we must first establish the conditions of the control inputs over the modes. 

\begin{itemize}
    \item \textit{Control consensus:} if timestep $k$ is a timestep in which control consensus is asserted over modes  - i.e. $\pU^i$=$\pU^j,  \forall i,j \in [1..M]$, then each control decision variable, $\pU_k^i$, has an identical feasible set
    \begin{equation}
        \mathcal{F}_k^* = \bigcap_{i=1}^M \mathcal{F}_k^i
    \end{equation}
    and the mode-joint feasible set is
    \begin{equation}
        \mathcal{F}_{k, \text{con}} = \{(\pU_k^1, \ldots, \pU_k^M) \in \mathbb{R}^{M\times m} \mid \pU_k^i \in \mathcal{F}_k^*\}
    \end{equation}
    \zl{consistency for set notation}
        \item \textit{No control consensus:} if timestep $k$ is a timestep in which control consensus is not asserted, then:
    % \begin{equation}
    %     \mathcal{F}_k = \bigcup_{i=1}^M \mathcal{F}_k^i
    % \end{equation}
    
    \begin{equation}
        \mathcal{F}_{k, \text{ind}} = \prod_{i=1}^M \mathcal{F}_k^i
    \end{equation}
\end{itemize}

Therefore, $\mathcal{F}_{k,\text{con}} \subseteq \mathcal{F}_{k,\text{ind}}$. \qh{This is only true in certain cases, e.g., if timestep $k$ is the first time step in which there is no consensus.}
\end{proof}
This shows that at a given horizon step $k$ the feasible set of the Problem \ref{prob:safetrajectoryplanning} is equivalent or smaller if consensus is asserted.

\begin{theorem}
    The feasible control set for Problem \ref{prob:safetrajectoryplanning} under a consensus horizon $h_1=H$ is smaller than the feasible control set under $h_2<H$.\qh{We should be able to generalize the theorem to the case for $h_1 < h_2 \leq H$} \RM{Agree}
    \label{thm:feasible}
\end{theorem}
\begin{proof}
    Consider two controllers \textit{A} and \textit{B} that solve Problem \ref{prob:safetrajectoryplanning}. Let the consensus horizon $h_1<H$. Then, 
    \begin{equation}
        \mathcal{F}_{k, \text{con}}^A=\mathcal{F}_{k, \text{con}}^B , \forall k\leq h_1. 
    \end{equation}
    
    Now let \textit{A} adopt $h_2=H$. Restricting the modes to be the same for $k>h_1$ can only reduce the size of $\mathcal{F}_{k, \text{con}}^A$ $\forall k\leq h_1$. Then,
    \begin{equation}
        \mathcal{F}_{k, \text{con}}^A\subseteq\mathcal{F}_{k, \text{con}}^B , \forall k\leq h_1.
    \end{equation}

    Now consider the reachable sets for \textit{A} and \textit{B} 
    \begin{align}
        \mathcal{R}_k^{i,A} = \{\pX_{t+k}^i \in \mathbb{R}^{n}: \pX_{t+k}^i = A_i\pX^i_k + B_i \pU_k, \pU_k \in \mathcal{F}_k^{*,A}\} \\
        \mathcal{R}_k^{i,B} = \{\pX_{t+k}^i \in \mathbb{R}^{n}: \pX_{t+k}^i = A_i\pX^i_k + B_i \pU_k, \pU_k \in \mathcal{F}_k^{*,B}\}.
     \end{align}

    We know that $\mathcal{R}_k^{i,A} \subseteq \mathcal{R}_k^{i,B}$ since $\mathcal{F}_k^{*,A} \subseteq \mathcal{F}_k^{*,B}$. Then, using Lemma \ref{lemma1}, 

    \begin{equation}
        \mathcal{F}_{k, \text{con}}^A\subseteq\mathcal{F}_{k, \text{ind}}^B, \forall k > h_1. 
    \end{equation}

    Finally, it follows that
    \begin{equation}
        \prod_{k=1}^{h_{1}}\mathcal{F}_k^A \subseteq \prod_{k=1}^{h_{2}}\mathcal{F}_k^B.
    \end{equation}
    
\end{proof}

Theorem \ref{thm:feasible} shows that for a higher consensus horizon, Problem \ref{prob:safetrajectoryplanning} may become infeasible. On the other hand, as discussed, too low of a consensus horizon may lead to unsafe behavior. This provides us with a \emph{robustness-feasibility trade-off}, where enforcing a longer consensus horizon leads to more robust (safe) control behavior, but may lead to an infeasible problem. 

\begin{theorem}
    At every planning instance of Problem~\ref{prob2:carriedconstraints} at time step $t$, there exists a $h^*$ such that safety is maximized and that maximizes the number of time steps in which the problem is guaranteed to be feasible.
\end{theorem}
